# Supplementary material for: The Influence of Prior Discourse on Conversational Agent-Driven Decision-Making
Source: arXiv:2503.04692 source file (2025-03-06)
Supplement: Supplementary file 1 [file all_decision_scenarios.tex]

\section{Decision Scenarios}
\label{sec:appendix-ds}
\subsection{Budget Allocation}
\label{sec:appendix-ds-ba}
\subsubsection{Neutral Condition}
\label{sec:appendix-ds-ba-neut1}

\begin{quote}
The National Highway Safety Commission is deciding how to allocate its budget between two safety research programs:
\begin{enumerate}
    \item Improving automobile safety (bumpers, body, gas tank configuration, seat-belts), and
    \item Improving the safety of interstate highways (guard rails, grading, highway interchanges, and implementing selective reduced speed limits).
\end{enumerate}

Since there is a ceiling on its total spending, it must choose between the options provided below. If you had to make this choice, which of the following will you choose?
 \begin{itemize}
     \item Allocate 60\% to auto safety and 40\% to highway safety
     \item Allocate 50\% to auto safety and 50\% to highway safety
 \end{itemize}
\end{quote}

\subsubsection{Neutral Condition - Alternative Swapped}
\label{sec:appendix-ds-ba-neut2}

\begin{quote}

The National Highway Safety Commission is deciding how to allocate its budget between two safety research programs:
\begin{enumerate}
    \item Improving automobile safety (bumpers, body, gas tank configuration, seat-belts), and
    \item Improving the safety of interstate highways (guard rails, grading, highway interchanges, and implementing selective reduced speed limits).
\end{enumerate}

Since there is a ceiling on its total spending, it must choose between the options provided below. If you had to make this choice, which of the following will you choose?
 \begin{itemize}
     \item Allocate 50\% to auto safety and 50\% to highway safety.
     \item Allocate 60\% to auto safety and 40\% to highway safety.
 \end{itemize}

\end{quote}

\subsubsection{Status Quo - 60A40H }
\label{sec:appendix-ds-ba-sq60a40h}

\begin{quote}

The National Highway Safety Commission is deciding how to allocate its budget between two safety research programs:
\begin{enumerate}
    \item Improving automobile safety (bumpers, body, gas tank configuration, seat-belts)
    \item Improving the safety of interstate highways (guard rails, grading, highway interchanges, and implementing selective reduced speed limits).
\end{enumerate}

Currently, the commission allocates approximately 60\% of its funds to auto safety and 40\% of its funds to highway safety.
Since there is a ceiling on its total spending, it must choose between the options provided below. If you had to make this choice, which of the following will you choose?
 \begin{itemize}
     \item Maintain present budget amounts for the programs.
     \item Decrease auto program by 10\% and raise highway program by like amount.
 \end{itemize}
    
\end{quote}

\subsubsection{Status Quo - 50A50H }
\label{sec:appendix-ds-ba-sq50a50h}

\begin{quote}

The National Highway Safety Commission is deciding how to allocate its budget between two safety research programs: 
\begin{enumerate}
    \item Improving automobile safety (bumpers, body, gas tank configuration, seat-belts)
    \item Improving the safety of interstate highways (guard rails, grading, highway interchanges, and implementing selective reduced speed limits).
\end{enumerate}

Currently, the commission allocates approximately 50\% of its funds to auto safety and 50\% of its funds to highway safety.
Since there is a ceiling on its total spending, it must choose between the options provided below. If you had to make this choice, which of the following will you choose? 

 \begin{itemize}
     \item Maintain present budget amounts for the programs.
     \item Increase auto program by 10\% and lower highway program by like amount.
 \end{itemize}

\end{quote}

\subsection{Investment Decision Making}
\label{sec:appendix-ds-idm}

\subsubsection{Neutral Condition}
\label{sec:appendix-ds-idm-neut1}

\begin{quote}

You are a serious reader of the financial pages but until recently have had few funds to invest. That is when you inherited a large sum of money from your great uncle. You are considering different portfolios.
Your choices are:
 \begin{itemize}
     \item Invest in moderate-risk Company A. Over a year's time, the stock has .5 chance of increasing 30\% in value, a .2 chance of being unchanged, and a .3 chance of declining 20\% in value.
     \item Invest in high-risk Company B. Over a year's time, the stock has a .4 chance of doubling in value, a .3 chance of being unchanged, and a .3 chance of declining 40\% in value.
 \end{itemize}
    
\end{quote}

\subsubsection{Neutral Condition - Alternative Swapped}
\label{sec:appendix-ds-idm-neut2}

\begin{quote}

You are a serious reader of the financial pages but until recently have had few funds to invest. That is when you inherited a large sum of money from your great uncle. You are considering different portfolios.
Your choices are:
 \begin{itemize}
     \item Invest in high-risk Company B. Over a year's time, the stock has a .4 chance of doubling in value, a .3 chance of being unchanged, and a .3 chance of declining 40\% in value.
     \item Invest in moderate-risk Company A. Over a year's time, the stock has .5 chance of increasing 30\% in value, a .2 chance of being unchanged, and a .3 chance of declining 20\% in value.
 \end{itemize}

\end{quote}

\subsubsection{Status Quo - Moderate Risk}
\label{sec:appendix-ds-idm-modrisk}

\begin{quote}
    You are a serious reader of the financial pages but until recently have had few funds to invest. That is when you inherited a portfolio of cash and securities from your great uncle. A significant portion of this portfolio is invested in moderate-risk Company A. You are deliberating whether to leave the portfolio intact or change it by investing in other securities. (The tax and broker commission consequences of any change are insignificant.)
Your choices are:
 \begin{itemize}
     \item Retain the investment in moderate-risk Company A. Over a year's time, the stock has .5 chance of increasing 30\% in value, a .2 chance of being unchanged, and a .3 chance of declining 20\% in value.
     \item Invest in high-risk Company B. Over a year's time, the stock has a .4 chance of doubling in value, a .3 chance of being unchanged, and a .3 chance of declining 40\% in value.
 \end{itemize}
\end{quote}

\subsubsection{Status Quo - High Risk}
\label{sec:appendix-ds-idm-highrisk}

\begin{quote}
    You are a serious reader of the financial pages but until recently have had few funds to invest. That is when you inherited a portfolio of cash and securities from your great uncle. A significant portion of this portfolio is invested in high-risk Company B. You are deliberating whether to leave the portfolio intact or change it by investing in other securities. (The tax and broker commission consequences of any change are insignificant.)
Your choices are:
 \begin{itemize}
     \item Retain the investment in high-risk Company B. Over a year's time, the stock has a .4 chance of doubling in value, a .3 chance of being unchanged, and a .3 chance of declining 40\% in value.
     \item Invest in moderate-risk Company A. Over a year's time, the stock has a .5 chance of increasing 30\% in value, a .2 chance of being unchanged, and a .3 chance of declining 20\% in value.
 \end{itemize}
\end{quote}

\subsection{College Jobs}
\label{sec:appendix-ds-cj}

\subsubsection{Neutral Condition}
\label{sec:appendix-ds-cj-neut1}

\begin{quote}
    Having just completed your graduate degree, you have two offers of teaching jobs in hand.
When evaluating teaching job offers, people typically consider the salary, the reputation of the school, the location of the school, and the likelihood of getting tenure (tenure is permanent job contract that can only be terminated for cause or under extraordinary circumstances).
Your choices are:
 \begin{itemize}
     \item College A: east coast, very prestigious school, high salary, fair chance of tenure.
     \item College B: west coast, low prestige school, high salary, good chance of tenure.
 \end{itemize}
\end{quote}

\subsubsection{Neutral Condition - Alternative Swapped}
\label{sec:appendix-ds-cj-neut2}

\begin{quote}
    Having just completed your graduate degree, you have two offers of teaching jobs in hand.
When evaluating teaching job offers, people typically consider the salary, the reputation of the school, the location of the school, and the likelihood of getting tenure (tenure is permanent job contract that can only be terminated for cause or under extraordinary circumstances).
Your choices are:
 \begin{itemize}
     \item College B: west coast, low prestige school, high salary, good chance of tenure.
     \item College A: east coast, very prestigious school, high salary, fair chance of tenure.
 \end{itemize}
\end{quote}

\subsubsection{Status Quo - College A}
\label{sec:appendix-ds-cj-colla}
You are currently an assistant professor at College A in the east coast. Recently, you have been approached by colleague at other university with job opportunity.
When evaluating teaching job offers, people typically consider the salary, the reputation of the school, the location of the school, and the likelihood of getting tenure (tenure is permanent job contract that can only be terminated for cause or under extraordinary circumstances).
Your choices are:
 \begin{itemize}
     \item Remain at College A: east coast, very prestigious school, high salary, fair chance of tenure.
     \item Move to College B: west coast, low prestige school, high salary, good chance of tenure.
 \end{itemize}
\begin{quote}
    
\end{quote}

\subsubsection{Status Quo - College B}
\label{sec:appendix-ds-cj-collb}
You are currently an assistant professor at College B in the west coast. Recently, you have been approached by colleague at other university with job opportunity.
When evaluating teaching job offers, people typically consider the salary, the reputation of the school, the location of the school, and the likelihood of getting tenure (tenure is permanent job contract that can only be terminated for cause or under extraordinary circumstances). 
Your choices are:
 \begin{itemize}
     \item Remain at College B: west coast, low prestige school, high salary, good chance of tenure.
     \item Move to College A: east coast, very prestigious school, high salary, fair chance of tenure.
 \end{itemize}
\begin{quote}
    
\end{quote}
