# Supplementary material for: The Influence of Prior Discourse on Conversational Agent-Driven Decision-Making
Source: arXiv:2503.04692 source file (2025-03-06)
Supplement: Supplementary file 2 [file complex_task_questions.tex]

\begin{longtable*}[c]{@{}ccccc@{}}
\toprule
\textbf{Domain} & \multicolumn{3}{c}{\textbf{Attribute}} & \textbf{Questions} \\* \midrule
\endfirsthead
\multicolumn{5}{c}%
{{\bfseries Table \thetable\ continued from previous page}} \\
\toprule
\textbf{Domain} & \multicolumn{3}{c}{\textbf{Attribute}} & \textbf{Questions} \\* \midrule
\endhead
\bottomrule
\endfoot
\endlastfoot
\textbf{\begin{tabular}[c]{@{}c@{}}Home \\ Property\end{tabular}} & \textbf{\begin{tabular}[c]{@{}c@{}}Number of \\ Bedrooms\end{tabular}} & \textbf{\begin{tabular}[c]{@{}c@{}}Size \\ (Sq ft.)\end{tabular}} & \textbf{Property Reviews} & \textbf{} \\* \midrule
1st & Three Rooms & 2000 & Four star & \begin{tabular}[c]{@{}c@{}}In the following scenario choose \\ from various property recommendations.\end{tabular} \\
2nd & Two times 1st & Same as first & Same as first & \begin{tabular}[c]{@{}c@{}}The first property has three bedrooms, \\ 2000 square feet, and a 4-star rating. \\ The second property has twice the number of\\  bedrooms and with the same size and rating. \\ Which one do you prefer, and why?\end{tabular} \\
3rd & Same as the second & Half of first & Same as first & \begin{tabular}[c]{@{}c@{}}The third property has the same \\ number of bedrooms as the second one \\ but is half the size of the first one,\\  with the same rating as the first. \\ Which one do you prefer, and why?\end{tabular} \\
4th & Same as the second & Same as third & \begin{tabular}[c]{@{}c@{}}One star less \\ than the first\end{tabular} & \begin{tabular}[c]{@{}c@{}}The fourth property has the same \\ number of bedrooms as the second, \\ the same size as the third, but \\ one less star rating than the first. \\ Which one do you prefer, and why?\end{tabular} \\
 &  &  &  & \begin{tabular}[c]{@{}c@{}}Remember the details \\ of the fourth property. \\ Specific information \\ will be requested later.\end{tabular} \\* \midrule
\textbf{\begin{tabular}[c]{@{}c@{}}Music\\ Artist\end{tabular}} & \textbf{\begin{tabular}[c]{@{}c@{}}Live \\ Performances\end{tabular}} & \textbf{\begin{tabular}[c]{@{}c@{}}Artist \\ Remuneration \\ for Show\end{tabular}} & \textbf{Artist-Specific} & \textbf{} \\* \midrule
1st & Three & 2000 Units & Four star & \begin{tabular}[c]{@{}c@{}}In the following scenario choose\\  from various artist recommendations.\end{tabular} \\
2nd & 2 times 1st & Same as first & Same as first & \begin{tabular}[c]{@{}c@{}}The first artist performs\\  three live shows, \\ is paid 2000 units per show, \\ and has a 4-star rating. \\ The second artist performs \\ twice as many shows, \\ with the same pay and rating. \\ Which artist do you prefer, and why?\end{tabular} \\
3rd & Same as the second & Half of first & Same as first & \begin{tabular}[c]{@{}c@{}}he third artist performs the same\\  number of shows as the second, \\ earns half the pay of the first artist, \\ but has the same rating as the first. \\ Which artist do you prefer, and why?\end{tabular} \\
4th & Same as the second & Same as third & \begin{tabular}[c]{@{}c@{}}One star less \\ than the first\end{tabular} & \begin{tabular}[c]{@{}c@{}}The fourth artist performs the \\ same number of shows as the second, \\ earns the same pay as the third, but \\ has two stars less than the first artist. \\ Which artist do you prefer, and why?\end{tabular} \\
 &  &  &  & \begin{tabular}[c]{@{}c@{}}Remember the \\ details of the fourth artist. \\ Specific information\\  will be requested later.\end{tabular} \\* \midrule
\textbf{\begin{tabular}[c]{@{}c@{}}Movies - \\ Streaming \\ Service\end{tabular}} & \textbf{\begin{tabular}[c]{@{}c@{}}Number of \\ Parallel Devices\end{tabular}} & \textbf{Library Size} & \textbf{Service Rating} & \textbf{} \\* \midrule
1st & Three & 2000 Movies & Four star & \begin{tabular}[c]{@{}c@{}}In the following scenario choose from \\ various streaming service recommendations.\end{tabular} \\
2nd & 2 times 1st & Same as first & Same as first & \begin{tabular}[c]{@{}c@{}}The first streaming service supports \\ 3 parallel devices, \\ has a library of 2000 movies,\\  and is rated 4 stars. \\ The second service supports \\ twice as many devices, \\ with the same library size and rating. \\ Which service do you prefer, and why?\end{tabular} \\
3rd & Same as the second & Half of first & Same as first & \begin{tabular}[c]{@{}c@{}}The third streaming service supports the\\  same number of devices as the second, has \\ half the library size of the first,\\  but has the same rating as the first. \\ Which service do you prefer, and why?\end{tabular} \\
4th & Same as the second & Same as third & \begin{tabular}[c]{@{}c@{}}One star less\\  than the first\end{tabular} & \begin{tabular}[c]{@{}c@{}}The fourth streaming service supports\\  the same number of devices as the second, \\ has the same library size as the third,\\  but is rated one star less than the first. \\ Which service do you prefer, and why?\end{tabular} \\
 &  &  &  & \begin{tabular}[c]{@{}c@{}}Remember the details of the fourth service. \\ Specific information will be requested later.\end{tabular} \\*
\midrule
\textbf{\begin{tabular}[c]{@{}c@{}}Calendar\\ App\end{tabular}} & \textbf{\begin{tabular}[c]{@{}c@{}}Calendar Syncing \\ Across Devices\end{tabular}} & \textbf{\begin{tabular}[c]{@{}c@{}}Managed \\ Tasks \\ Per Year\end{tabular}} & \textbf{\begin{tabular}[c]{@{}c@{}}Event Privacy \\ Rating\end{tabular}} & \textbf{} \\* 
\midrule
1st & 3 & 2000 & Four star & \begin{tabular}[c]{@{}c@{}}In the following scenario choose from \\ Various Apps recommendations for calendar.\end{tabular} \\
2nd & 2 times 1st & Same as first & Same as first & \begin{tabular}[c]{@{}c@{}}The first calendar app can sync\\  across three devices, \\ manages 2000 tasks per year,\\  and has a 4-star privacy rating. \\ The second app syncs across two devices, \\ manages the same number of tasks,\\  and has the same privacy rating. \\ Which app do you prefer, and why?\end{tabular} \\
3rd & Same as Second & Half of first & Same as first & \begin{tabular}[c]{@{}c@{}}The third app syncs across the same\\  number of devices as the second app, \\ but manages half as\\  many tasks as the first app, \\ with the same privacy rating as the first. \\ Which app do you prefer, and why?\end{tabular} \\
4th & Same as Second & Same as third & \begin{tabular}[c]{@{}c@{}}One star less\\  than the first\end{tabular} & \begin{tabular}[c]{@{}c@{}}The fourth app syncs across the same number \\ of devices as the second, manages the same\\  number of tasks as the third, but has one less \\ star in privacy rating compared to the first. \\ Which app do you prefer, and why?\end{tabular} \\
 &  &  &  & \begin{tabular}[c]{@{}c@{}}Remember the details of the fourth App. \\ Specific information will be requested later.\end{tabular} \\* 
 
 \midrule
\textbf{Bank} & \textbf{\begin{tabular}[c]{@{}c@{}}Bank Branch \\ Proximity\end{tabular}} & \textbf{Interest Rates} & \textbf{\begin{tabular}[c]{@{}c@{}}Fee-Free \\ Accounts\\  Rating\end{tabular}} & \textbf{} \\* 
\midrule
1st & 3km & 2000 units & Four & \begin{tabular}[c]{@{}c@{}}In the following scenario choose \\ from various banks recommendations.\end{tabular} \\
2nd & 2 times 1st & Same as first & Same as first & \begin{tabular}[c]{@{}c@{}}The first bank is 3 km away,\\  offers 2000 units of interest, \\ and has a four-star rating for fee-free accounts. \\ The second bank is twice as far away, \\ offers the same amount of interest,\\  and has the same fee-free account rating. \\ Which bank would you prefer, and why?\end{tabular} \\
3rd & Same as the second & Half of first & Same as first & \begin{tabular}[c]{@{}c@{}}The third bank is as far away as the second bank, \\ offers half the amount of interest as \\ the first bank, but has the same fee-free\\  account rating as the first bank. \\ Which bank would you prefer, and why?\end{tabular} \\
4th & Same as the second & Same as third & \begin{tabular}[c]{@{}c@{}}One star less \\ than the first\end{tabular} & \begin{tabular}[c]{@{}c@{}}The fourth bank is as far\\  away as the second bank, \\ offers the same amount of interest as the third bank, \\ but has one star less in fee-free account rating\\  compared to the first bank. \\ Which bank would you prefer, and why?\end{tabular} \\*

\midrule
\textbf{\begin{tabular}[c]{@{}c@{}}Messaging \\ App\end{tabular}} & 
\textbf{\begin{tabular}[c]{@{}c@{}}Number of \\ Simultaneous \\Devices\end{tabular}} & 
\textbf{\begin{tabular}[c]{@{}c@{}}Messages \\ Per Day\end{tabular}} & 
\textbf{\begin{tabular}[c]{@{}c@{}}Security \\ Rating\end{tabular}} & 
\textbf{} \\* 
\midrule

1st & 3 & 2000 & Four star & 
\begin{tabular}[c]{@{}c@{}}In the following scenario, choose from \\ various messaging app recommendations.\end{tabular} \\ 
2nd & 2 times 1st & Same as first & Same as first & 
\begin{tabular}[c]{@{}c@{}}The first messaging app allows access \\ on three devices, supports 2000 messages per day, \\ and has a 4-star security rating. \\ The second app allows access on\\ twice as many devices, \\ supports the same number of messages, \\ and has the same security rating. \\ Which app do you prefer, and why?\end{tabular} \\ 
3rd & Same as the second & Half of first & Same as first & 
\begin{tabular}[c]{@{}c@{}}The third app allows access on the same \\ number of devices as the second app, \\ but supports half as many messages as the first app, \\ with the same security rating as the first. \\ Which app do you prefer, and why?\end{tabular} \\ 
4th & Same as the second & Same as third & One star less than the first & 
\begin{tabular}[c]{@{}c@{}}The fourth app allows access on the \\ same number of devices as the second, \\ supports the same number \\ of messages as the third, \\ but has one less star in \\security rating compared to the first. \\ Which app do you prefer, and why?\end{tabular} \\ 
& & & & 
\begin{tabular}[c]{@{}c@{}}Remember the details\\ of the fourth app, \\ including the number\\ of devices, messages per day, \\ and its security rating.\\ Specific information \\ will be requested later.\end{tabular} \\* 
% \bottomrule

\caption{Complex Tasks for prior discourse.}
\label{tab:my-table}\\
\end{longtable*}
