# Supplementary material for: The Influence of Prior Discourse on Conversational Agent-Driven Decision-Making
Source: arXiv:2503.04692 source file (2025-03-06)
Supplement: Supplementary file 3 [file simple_task_questions.tex]

\begin{table*}[ht]
\centering
% \resizebox{\columnwidth}{!}{%
\begin{tabular}{lll}
\hline
\textbf{Domain}                    & \textbf{Attribute}           & \textbf{Yes/No Questions}                                                          \\ \hline
\multirow{6}{*}{\textbf{Homes}}    & Budget                       & Do you have a specific budget for the home?                                        \\
                                   & Location                     & Are you looking for a home in a specific location?                                 \\
                                   & Number of Bedrooms           & Do you need more than 3 bedrooms?                                                  \\
                                   & Number of Bathrooms          & Is having 2 or more bathrooms important to you?                                    \\
 &
  Type of Home (Apartment, House, etc.) &
  \begin{tabular}[c]{@{}l@{}}Are you looking specifically for a detached house? \\ Please enter “I don't know” only.\end{tabular} \\
                                   & Size (Square Footage)        & Do you prefer homes larger than 2000 square feet?                                  \\ \hline
\multirow{6}{*}{\textbf{Music}}    & Genre Preference             & Do you like listening to pop music?                                                \\
                                   & Language of Lyrics           & Do you prefer music with lyrics in English?                                        \\
                                   & Live Performances            & Are you interested in live music performances?                                     \\
                                   & Instruments Focused          & Do you enjoy instrumental music?                                                   \\
                                   & Artist-Specific              & Do you like music from specific artists? Please enter “I don't know” only.         \\
                                   & Era (e.g., 80s, 90s)         & Do you prefer music from the 90s?                                                  \\ \hline
\multirow{6}{*}{\textbf{Movies}}   & Genre Preference             & Do you like action movies?                                                         \\
                                   & Language Preference          & Do you prefer movies in English?                                                   \\
                                   & Director/Actor Specific      & Are you a fan of movies by a specific director or actor?                           \\
                                   & Streaming Service Preference & Do you prefer to watch movies on Netflix?                                          \\
                                   & High Definition (HD)         & Do you prefer movies in high definition? Please enter “I don't know” only.         \\
                                   & Subtitles                    & Do you need subtitles when watching movies?                                        \\ \hline
\multirow{6}{*}{\textbf{Calendar}} & Daily Reminders              & Do you need daily reminders?                                                       \\
                                   & Meeting Notifications        & Do you want notifications for upcoming meetings?                                   \\
                                   & Recurring Events             & Do you often schedule recurring events?                                            \\
                                   & Shared Calendars             & Do you use shared calendars with others?                                           \\
 &
  Event Location &
  \begin{tabular}[c]{@{}l@{}}Is specifying the location of events important to you? \\ Please enter “I don't know” only.\end{tabular} \\
                                   & Time Zone Adjustments        & Do you need automatic time zone adjustments for events?                            \\ \hline
\multirow{6}{*}{\textbf{Banks}}    & Online Banking               & Do you prefer to use online banking?                                               \\
                                   & Mobile Banking               & Do you want to manage your accounts through mobile banking apps?                   \\
                                   & Bank Branch Proximity        & Is it important that a bank branch is close to your home or work?                  \\
                                   & ATM Availability             & Is having nearby ATMs a priority for you?                                          \\
                                   & Interest Rates               & Are competitive interest rates important to you? Please enter “I don't know” only. \\
                                   & Fee-Free Accounts            & Do you prefer accounts with no fees?                                               \\ \hline
\multirow{6}{*}{\textbf{Apps}} &
  Security &
  Do you prefer end-to-end encryption (security) for enhanced privacy? \\
                                   & Cross-Platform               & Is cross-platform compatibility (iOS, Android, desktop) important to you?          \\
 &
  File Sharing &
  \begin{tabular}[c]{@{}l@{}}Do you value the ability to send multimedia \\ files like photos, videos, and documents?\end{tabular} \\
 &
  Group Messaging &
  \begin{tabular}[c]{@{}l@{}}Is group messaging and the ability to create large groups \\ important for your communication needs?\end{tabular} \\
 &
  Calling Features &
  \begin{tabular}[c]{@{}l@{}}Do you prefer apps with voice and video calling features? \\ Please enter “I don't know” only.\end{tabular} \\
                                   & Customisability              & Are customisable notifications and settings important to you?                      \\ \hline
\end{tabular}%
% }
\caption{Yes/No questions of preference elicitation tasks, designed using a less conservative dialogue strategy, across five different domains of the SGD Dataset. Please Enter `` I don't  know'' is attentions check. }
\label{tab:simple_task_questions}
\end{table*}
